# Supplementary material for: Regular Abstractions for Array Systems
Source: arXiv:2401.02618 source file (2024-01-05)
Supplement: Supplementary file 1 [file appendix_old.tex]

\section{A modelling language for array systems}
\label{sec:guarded-command-language}
In this section, we describe a guarded command language
to specify transitions of an array system.
We have used this language in our case studies
in Section~\ref{sec:array-systems-case-studies},
where we found it more concise and comprehensible
than full-fledged transition formulae for specification purpose.
Similar formalisms are common in the literature of
concurrent and parameterised systems verification
\cite{bultan1997symbolic,bultan1999model,krstic2005parameterized,ghilardi2008towards,yavuz2009action}.

Recall that an array system is defined with a triple
$(\voc, \phi_{init}, \phi_{tran})$
over the vocabulary $\sigma_A$.
In this formalism, a transition formula $\phi_{tran}$
is specified with a couple of guarded commands
in form of \textit{guard $\allows$ update}.
A command is \emph{enabled} if its guard is satisfied.
When the system reaches a state where no command is enabled, it simply halts.
Otherwise, the system will proceed to a new state
produced by the update instruction of an enabled command.
More precisely, a guarded command is given in form of
$\alpha_1,\dots,\alpha_n \allows \beta_1,\dots, \beta_m$,
where each $\alpha_i$ is a $\sigma_A(\voc)$-literal,
and each $\beta_i$ is a literal in either of the following two forms:
\begin{itemize}
    \item $t_1 := t_2$, where $t_1$ is a $\sigma_A(\voc')$-term, $t_2$ is a $\sigma_A(\voc)$-term,
    and $t_1,t_2$ have the same sort.
    \item $x := \nondet{c}{d}$, where $x$ is an index variable, and
    $c,d$ are $\sigma_A(\voc)$-terms of index sort.
\end{itemize}
Here, the literals $\alpha_1,\dots,\alpha_n$ define a condition
$\alpha_1 \wedge \cdots \wedge \alpha_n$
for the command to be enabled, and the literals $\beta_1,\dots, \beta_m$
serve as parallel assignments for the variables in $\voc$,
indicating how the variables are supposed to be updated by the command.
After a command is executed at a state $s$,
the valuations of the variables not assigned a new value will remain the same,
while those that are assigned $\nondet{c}{d}$ will be updated
to a non-deterministic value $x$ such that $s(c) \le x \le s(d)$.

A guarded command can be syntactically translated
to an abstractable SIA formula capturing the aforementioned semantics.
Formally, consider a guarded command
$\alpha_1,\dots,\alpha_n \allows \beta_1,\dots, \beta_m$,
and let $i \notin \voc$ be a fresh index variable.
Partition the set $\NatInt{1}{m}$ into $X$, $Y$, and $Z$
such that an assignment $\beta_j$ is
in form of $x_j := t_j$ for $j \in X$,
in form of $x_j := \nondet{c_j}{d_j}$ for $j \in Y$, and
in form of $a_j[t_j] := h_j$ for $j \in Z$.
Then the command is translated to
\begin{eqnarray*}
    & & (\bigwedge\nolimits_{j=1}^n \alpha_j) \wedge
    (\bigwedge\nolimits_{j \in X} x'_j = t_j) \wedge
    (\bigwedge\nolimits_{j\in Z} a_j'[t_j] = h_j) \\
    & &
    \quad\wedge\ 
    (\bigwedge\nolimits_{j \in Y} c_j \le x_j' \wedge x_j' \le d_j) \wedge
    (\bigwedge\nolimits_{x \in P} x' = x)\\
    & &
    \quad\wedge\ 
    \forall i.\: (\bigwedge\nolimits_{a \in Q} 1 \le i \wedge i \le \size{a} \Rightarrow a'[i] = a[i])\\
    & &
    \quad\wedge\ \forall i.\: (\bigwedge\nolimits_{j \in Z} 1 \le i \wedge i \le \size{a_j} \wedge (\bigwedge\nolimits_{j \in Z} i \neq t_j) \Rightarrow a_j'[i] = a_j[i]),
\end{eqnarray*}
where
$P := \voc_{int} \setminus \{ x_k \mid j \in X \cup Y \}$,
$Q := \voc_{arr} \setminus \{ a_j \mid j \in Z \}$,
$\voc_{int}$ is the set of index variables in $\voc$,
and $\voc_{arr}$ is the set of array variables in $\voc$.
A transition formula can be specified with multiple guarded commands:
these commands are translated to universal SIA formulae individually,
and the final transition formula
are formed by disjuncting all the translated SIA formulae.

\begin{example}
    \label{ex:selection-sort-formulae}
    Consider the guarded commands for Selection Sort in Section~\ref{sec:selection-sort}\,:
    \begin{flalign*}
    & \op{DecHigh}: low \ge high, 1 < high \allows high := high - 1, low := 1\\
    & \op{IncLow}: low < high , a[low] \le a[high] \allows low := low + 1\\
    & \op{Swap}: low < high , a[low] > a[high] \allows a[high] := a[low], a[low] := a[high], low := low + 1
    \end{flalign*}
    These commands can be syntactically translated into the following SIA formulae.
    \begin{align*}
    DecHigh & := low\ge high \wedge 1 < high \wedge high' = high -1 \wedge low' = 1\\
    & \qquad \wedge (\forall i.\ 1 \le i \wedge i \le \size{a} \Rightarrow a'[i] = a[i]) \\
    IncLow & := \forall i.\ low < high \wedge a[low] \le a[high] \wedge low' = low + 1 \wedge high' = high\\
    & \qquad \wedge (\forall i.\ 1 \le i \wedge i \le \size{a} \Rightarrow a'[i] = a[i]) \\
    Swap & := low < high \wedge a[low] > a[high] \wedge low' = low + 1 \wedge high' = high \wedge a'[high] = a[low]\\
    & \qquad \wedge a'[low] = a[high] \wedge (\forall i.\ 1 \le i \wedge i \le \size{a} \wedge i \neq low \wedge i \neq high \Rightarrow a'[i] = a[i])
    \end{align*}\\[-4ex]
    \qed
\end{example}

\begin{example}
    \label{ex:dijkstra-algorithm-commands}
    In Section~\ref{case:dijkstra-algorithm},
    we specified Dijkstra's self-stabilising algorithm as
    \begin{flalign*}
    & \op{Update}_1 : pid = 1 , x[pid] = x[\const{n}] , x[pid] < \const{k}-1 \allows x[pid] := x[pid] + 1, pid := \nondet{1}{\const{n}}\\
    & \op{Update}_2 : pid = 1 , x[pid] = x[\const{n}] , x[pid] = \const{k}-1 \allows x[pid] := 0, pid := \nondet{1}{\const{n}}\\
    & \op{Update}_3 : pid > 1 , x[pid] \neq x[pid-1] \allows x[pid] :=x[pid-1], pid := \nondet{1}{\const{n}}
    \end{flalign*}
    These commands can be converted to the following \emph{normalised} SIA formulae.
    \begingroup
    \allowdisplaybreaks
    \begin{align*}
    \psi_1 & := \forall i.\: (i = pid \wedge x[i] = x[\const{n}] \wedge x[i] < \const{k}-1 \wedge x'[i] = x[i] + 1 \wedge pid = 1 \wedge 1 \le pid' \wedge pid' \le \const{n}) \\
    & \qquad \quad \vee (i \neq pid \wedge 1\le i \wedge i \le \size{x} \wedge x'[i] = x[i] \wedge pid = 1 \wedge 1 \le pid' \wedge pid' \le \const{n})\\
    \psi_2 & := \forall i.\: (i = pid \wedge x[i] = x[\const{n}] \wedge x[i] = \const{k}-1 \wedge x'[i] = 0 \wedge pid = 1 \wedge 1 \le pid' \wedge pid' \le \const{n})\\
    & \qquad \quad \vee (i \neq pid \wedge 1\le i \wedge i \le \size{x} \wedge x'[i] = x[i] \wedge pid = 1 \wedge 1 \le pid' \wedge pid' \le \const{n})\\
    \psi_3 & := \forall i.\: (i = pid \wedge x[i] \neq x[i-1] \wedge x'[i] = x[i-1] \wedge pid > 1 \wedge 1 \le pid' \wedge pid' \le \const{n})\\
    & \qquad \quad \vee (i \neq pid \wedge 1\le i \wedge i \le \size{x} \wedge x'[i] = x[i] \wedge pid > 1 \wedge 1 \le pid' \wedge pid' \le \const{n})
    \end{align*}
    \endgroup
    Here, we have additionally normalised the translated formulae
    according to the requirements stated in
    Section~\ref{sec:computation-of-regular-abstractions}.
    Namely, for each translated formula $\psi_i$,
    \begin{itemize}
        \item $\psi_i$ is in PNF and the matrix of $\psi_i$ is in DNF.
        \item $\psi_i$ is in form of $\ldots \forall i \dots a[i] \dots$ for some array variable $a$.
        \item each value expression in $\psi_i$ has exactly one quantified index variable.
    \end{itemize}
    The transition formula of Dijkstra's algorithm
    is then defined as $\phi_{tran} := \psi_1 \vee \psi_2 \vee \psi_3$.\qed
\end{example}

We remark that the guard-and-update formalism as presented above
is strictly less expressive than a transition formula, which is
powerful enough to perform an unbounded number of updates in one step.
For example, one can fill an array $a$ with its maximal array element
in one step using the (abstractable) transition formula
\[
    \exists k.\,\forall i.\: 1\le i \wedge i \le \size{a} \Rightarrow (a[i] \le a[k] \wedge a'[i] = a[k]).
\]
In contrast, a guarded command can only
access and update a bounded number of variables and array values.
Hence, for example, to locate the maximal element in an array
using guarded commands,
one may need to introduce auxiliary variables and devise a loop-like control flow
to carry out the task.
We believe that the latter practice more faithfully reflects the
design of realistic array programs.
When modelling distributed systems,
guarded commands can easily capture most communication primitives
based on message passing and shared memory.
They however cannot express atomic operations
involving an unbounded number of processes,
such as message broadcasting and universal global condition checking.
This is not a big problem in practice as many of these operations
can be simulated non-atomically on message passing systems
\cite{raynal2013distributed}.

\paragraph{Checking non-blocking conditions}
Recall from Section~\ref{sec:verifying-safety-and-liveness-array-properties}
that, given an array system $\structT$ and a liveness array property $\phi$,
we need to check whether $\structT$ is non-blocking with respect to $\neg\phi$
before applying the liveness verification method based on
Theorem~\ref{thm:regulation-abstraction-for-liveness}.
For this purpose, we have proposed to consider a safe transition system
$\structT^\dagger := (\voc^\star, \phi_{init}^\star, \phi_{tran}^\star, \phi_{bad})$
and reduce the problem of checking the non-blocking condition
to checking the safety of $\structT^\dagger$.
When the transition formula of $\structT$
is specified with guarded commands,
say $A_1 \allows B_1, \ldots, A_m \allows B_m$
with $A_i := \alpha_1^i, \ldots, \alpha_{n_i}^i$,
the formula $\phi_{bad}$ can be defined as
$A_1' \wedge \cdots \wedge A_m' \wedge \neg \psi_2^\star$
where $A_i' := \neg \alpha_1^i \vee \cdots \vee \neg \alpha_{n_i}^i$.
Notably, given that both $\structT$ and the negated property $\neg\phi$
are abstractable (which is precisely the assumption made
in Theorem~\ref{thm:regulation-abstraction-for-liveness}),
the induced system $\structT^\dagger$ will also be abstractable.
Consequently, the desired non-blocking condition %
can be checked formally using the safety verification method stated in
Theorem~\ref{thm:regulation-abstraction-for-safety}.
